# Supplementary material for: Towards Natural Language-Based Visualization Authoring
Source: arXiv:2208.10947 source file (2022-10-23)
Supplement: Supplementary file 1 [file VIS_appendices.tex]

\section{Editing actions} \label{app:actions}

Operations may apply to different objects, depending on the properties of the objects. 
Table 1 lists the operations and the corresponding target objects and possible parameters. 
Operations are not exclusive because human languages may express same meanings with different patterns. For example, binding a data field to x axis, has the same effect as encode the horizontal position of mark to the field. Note the operations are not exhaustive.  

\begin{table*}[h]
    \centering
    \includegraphics[width=1\linewidth]{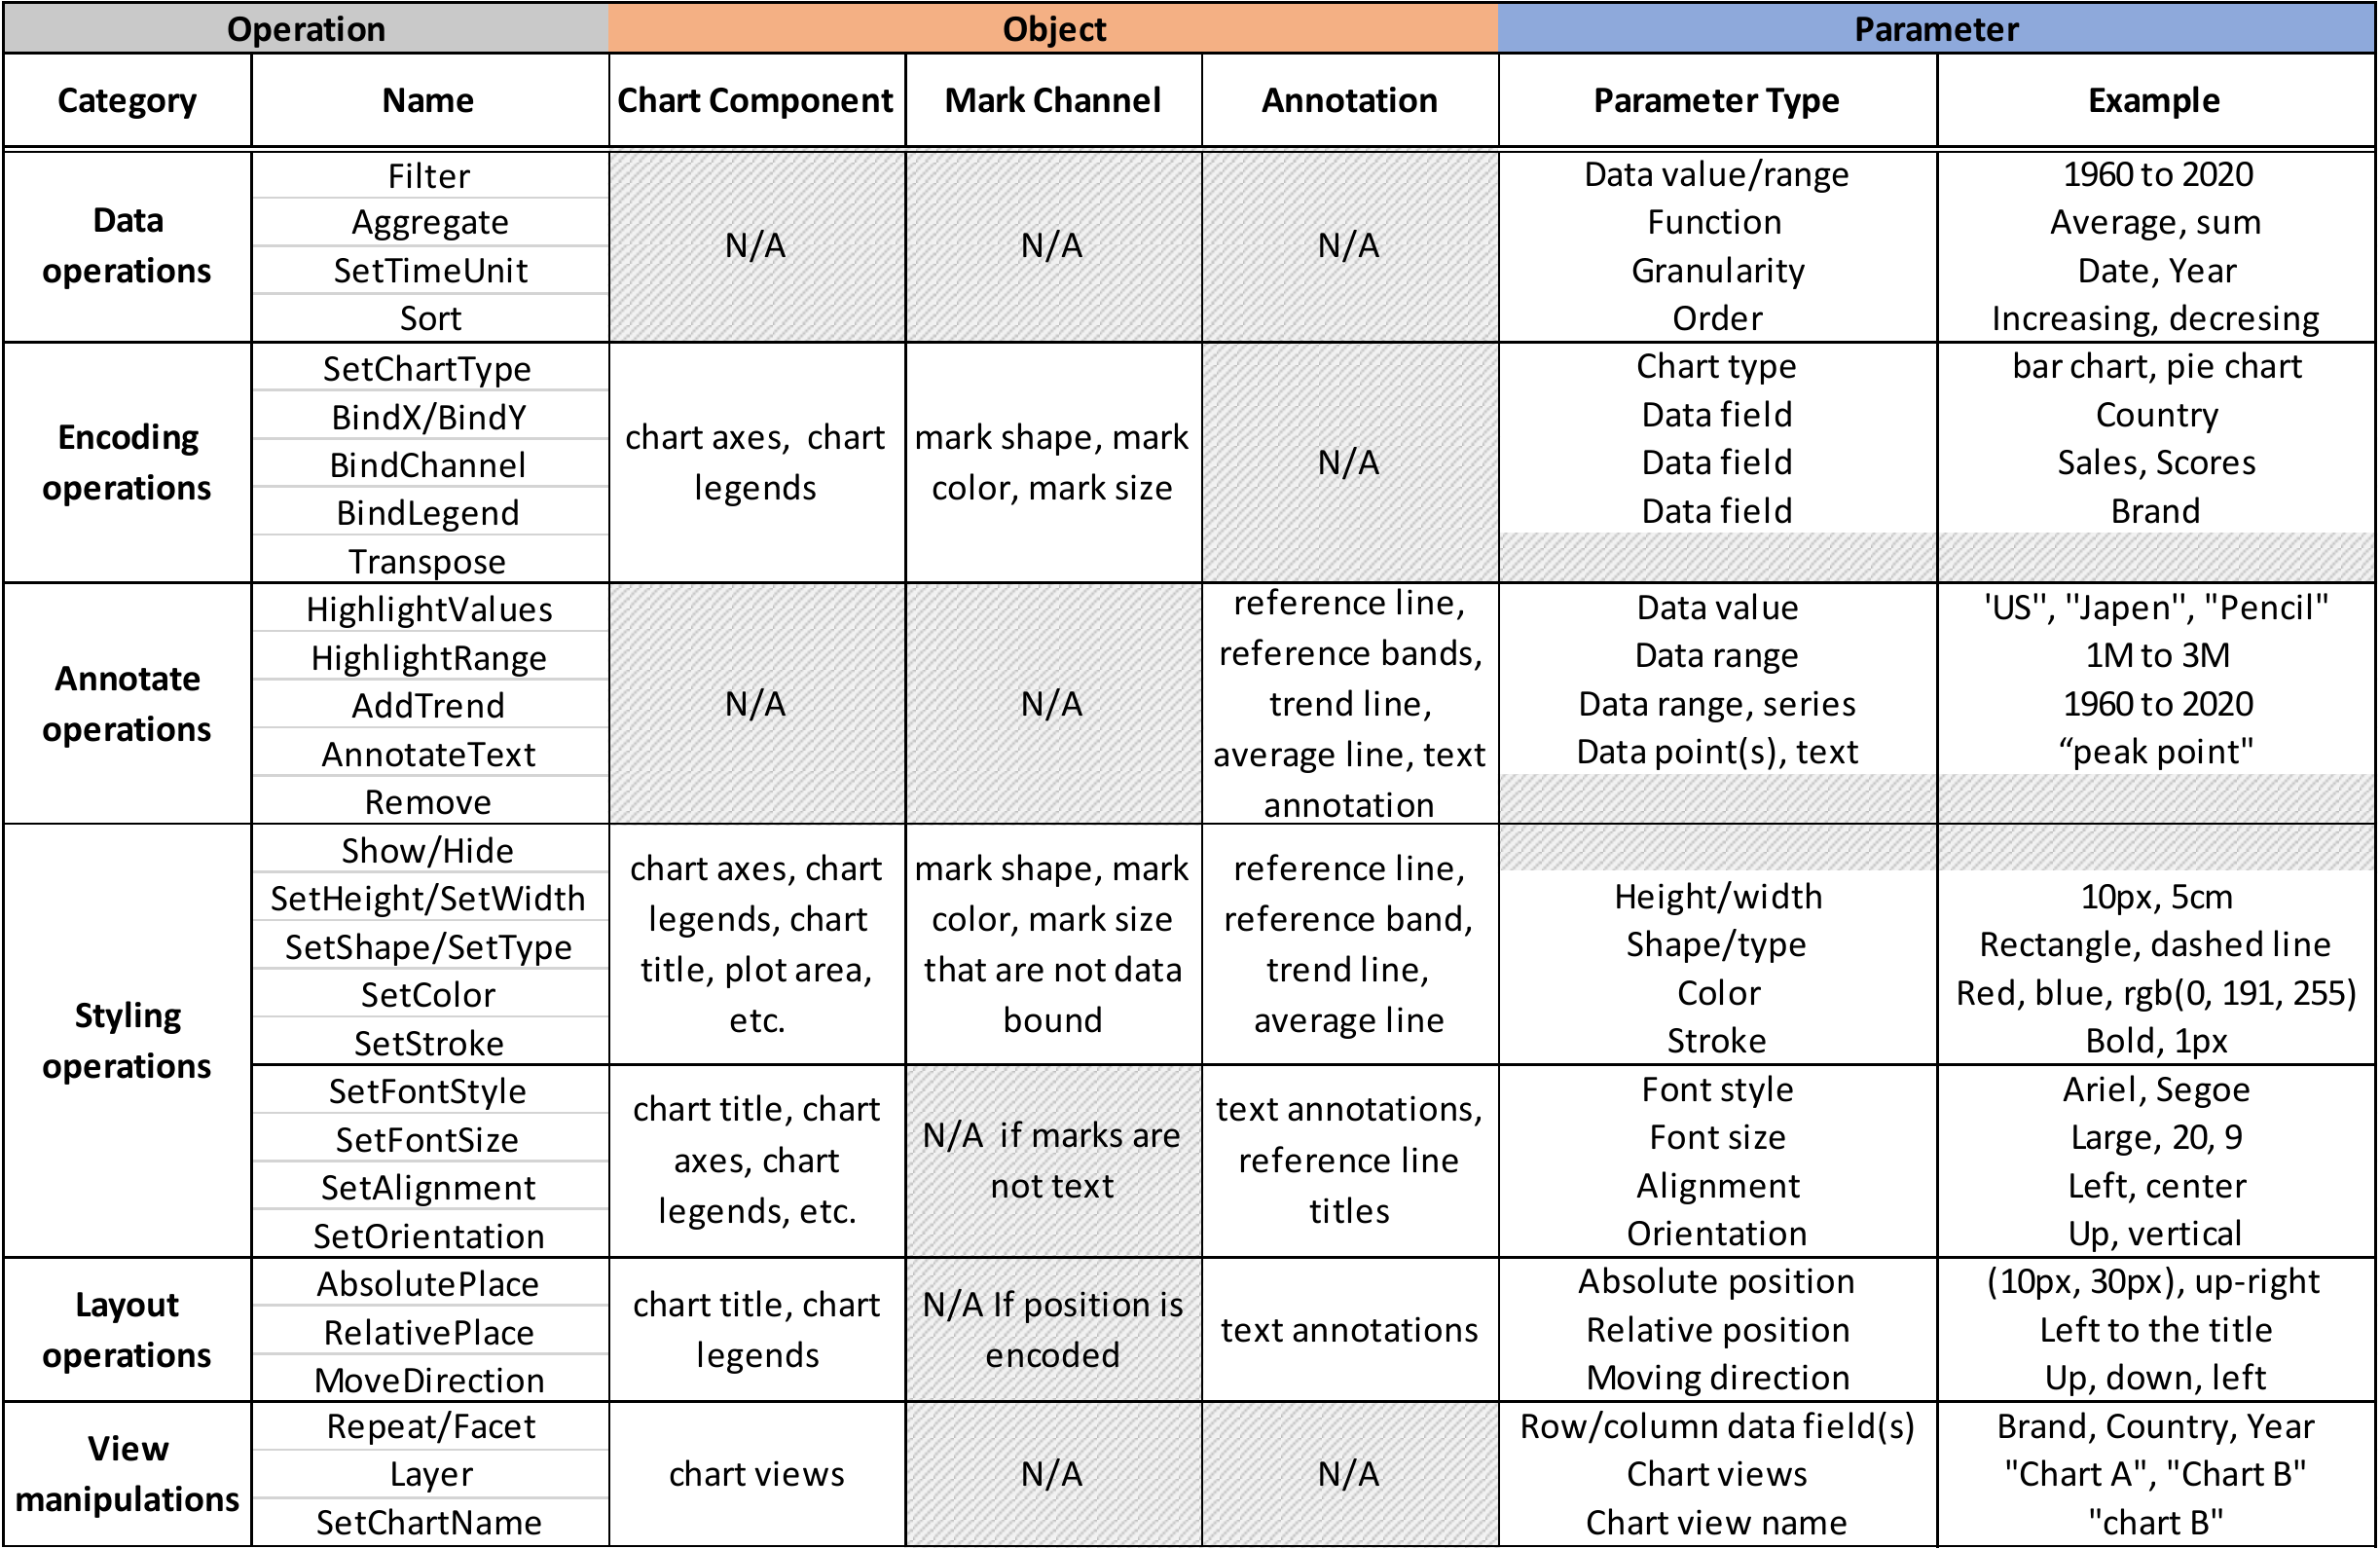}
    \vspace{0px}
    \caption{An authoring action consists of three parts, operation, object, and parameter. The table shows example authoring operations and the  corresponding objects and parameters. Operation are categorized into six major groups. Objects are categorized into chart components (e.g., axes, legends, title), mark channels (e.g., shape, color, size, position), and annotations (e.g., reference lines, reference bands, trend lines). }
    \label{fig:taxonomy1}
    \vspace{-1px}
\end{table*}
